# Supplementary material for: IDentity with Locality: An ideal hash for gene sequence search
Source: arXiv:2406.14901 source file (2024-06-21)
Supplement: Supplementary file 1 [file appendix.tex]

\clearpage
\onecolumn

\section{Proof of Theorem 1}
\begin{theorem} (general \name construction)
Let $\phi$ be drawn from a $(r_1, r_2, p_1, p_2)$ sensitive LSH family say $\mathcal{L}$ and $\rho_1, \rho_2$ be drawn from a random hash family, say $\mathcal{R}_1 : V \rightarrow [m], \mathcal{R}_2: U \rightarrow [L]$ respectively. Then the family of hash functions defined by 
\begin{equation}
    \mathcal{I} : \{\psi(x) = \rho_1(\phi(x)) + \rho_2(x)) \}
\end{equation}
is a $(r_1, r_2, \frac{L-1}{L}p_1, \frac{L}{m}+ p_2)$ sensitive and $L$ preserving {\longname } (\name) family.
\end{theorem}
If $d_U(x,y) \leq r_1$, then
\begin{proof}

\begin{align*}
    & \mathbf{Pr}(\mathbf{1}(\psi(x) \neq \psi(y)) \wedge d_V(x, y) < L ) \\
    & = \mathbf{Pr}(\phi(x) = \phi(y))\frac{L-1}{L} + \mathbf{Pr}(\phi(x) \neq \phi(y) \wedge (\textrm{satisfies the conditions}))\\
    & \geq \mathbf{Pr}(\phi(x) = \phi(y))\frac{L-1}{L} \\
    & = p_1 \frac{L-1}{L} 
\end{align*}

If $d_U(x,y) > r_2$, then,
\begin{align*}
    & \mathbf{Pr}( d_V(x, y) < L ) \\
    & = \mathbf{Pr}(\phi(x) = \phi(y)) + \mathbf{Pr}(\phi(x) \neq \phi(y) \wedge (\mathbf{Pr}(|\rho_1(x) - \rho_1(y)| < L) \wedge (\textrm{satisfies the condition}))\\
    & \leq p_2 + \mathbf{Pr}(\phi(x) \neq \phi(y) \wedge (\mathbf{Pr}(|\rho_1(x) - \rho_1(y)| < L)\\
    & \leq p_2 + (\mathbf{Pr}(|\rho_1(x) - \rho_1(y)| < L)\\
    & = p_2 + \frac{L}{m}\\
\end{align*}
\end{proof}

\section{Notations}
The notations used in the paper are as follows.
\begin{table}[h]
\centering
\caption{Notations used in the paper}
\label{tab:notations}
\begin{tabular}{|l|l|l|l|}
\hline 
notation & description & notation & description\\
\hline 
$m$ & range/ Bloom filter size & $\mathcal{L}$ & Family of LSH\\
\hline 
$n$ & number of insertions & $\mathcal{H}$ &Family of universal hash\\
\hline 
$\eta$ & number of hash in BF & $\mathcal{I}$  & Family of \name hash\\
\hline 
$x, y$ & keys/kmers & $\rho(.)$& random function\\
\hline 
$q$ & query kmer& $\phi(.)$& LSH hash function \\
\hline 
$Q$ & query gene & $\psi(.)$& \name hash function\\
\hline 
$G$ & whole gene & $\mathcal{S}(.)$& function string $\rightarrow$ Set\\
\hline 
$k$ & kmer size& $\mathcal{M}(.)$& MinHash\\
\hline 
$t$ & sub-kmer size& $\zeta(.), \ \mathcal{J}(.)$& Jaccard Similarity\\
\hline 
$N$ & number of files & $p_1,p_2$ & probabilities\\
\hline 
$T$ &  & $r_1,r_2$ & distances\\
\hline 
$L$ & IDL random hash range & $\mathbf{R}, \mathbf{N}$ & Real and Natural numbers \\
\hline
\end{tabular}
\end{table}

\section{Array of Bloom Filters for Multiple Set Membership Testing}
\begin{algorithm}
% \setstretch{1.14}
\begin{algorithmic}
\STATE {\bf INSERT: Array of \name-BF }
% $\psi: U\rightarrow m+L$: \name hash function
% $\rho :U \rightarrow [L]$ 
\STATE {\bf Input:} $\{G\}_{i =1}^{N}$: $N$ species genomes, $\{\mathbb{B}\}_{i =1}^{N}$: set of \name-BF 
\FOR{ $i \in 1..N$}
    \STATE $\mathbb{B}_i \leftarrow$ \name-BF INSERT($G_i$)\\
\ENDFOR
\STATE
\STATE {\bf QUERY: Array of \name-BF }
\STATE {\bf Input:} $Q$: query string, $\mathbb{B}_{i =1}^{N}$: Indexed set of \name-BF 
\STATE Init: Membership = $\mathbf{0}[N]$
\FOR{ $i \in 1..N$}
   \STATE Membership[$i$] = \name-BF QUERY($\mathbb{B}_i$)\\
\ENDFOR
 \end{algorithmic}
  \caption{Insert and query on Array of \name-BF}
  \label{alg:ABFInsertQuery}
\end{algorithm}

The State of the Art genome indices are based on the arrangement of Bloom filters. It was simply an Array with $O(N)$ query time \cite{bigSI, Bingmann2019COBSAC}. For reducing the order of complexity, other structures like a binary search tree type arrangement (Split Sequence Bloom Tree \cite{crainiceanu2013bloofi, SSBT}) or tabular arrangement (RAMBO \cite{gupta2021fast}), were also explored. All the data structures are a careful file insertion process in a set of Bloom filters, and hence can be generically seen as an array of bloom filters (ABF). Querying on these ABFs is called Multiple Set Membership Testing (MSMT).

MSMT tests whether a query is present in each of the sets. Algorithm \ref{alg:ABFInsertQuery} illustrates how \name-BF performs multiple set membership testing. We will compare \name-BF with the most popular and state-of-the-art solution for this problem, Array of Bloom Filters, which is a set of Bloom filters, one for each distinct set of items.
We randomly sample 100 files from the Whole Genome Sequencing data corpus and regard each file as a distinct set. For query generation, we randomly sample $10$ million subsequences of length $128$ from all $100$ files and perform a 1-poisoning (randomly file a basepair to an unknown character) attack on each subsequence.

Genomic datasets are huge, hence the ABF may not be able to fit in RAM as they can take up to Terabytes of memory. Real applications will require Bloom filters to reside on disk for large datasets to achieve desired accuracy and efficient query time. Therefore, we evaluated \name-BF for multiple set membership testing in two scenarios, when the data structure resides in RAM and when it resides on disk. Disk access is usually orders of magnitude slower than RAM access, therefore it poses a significant bottleneck with page faults.

\section{Analysing False positive rate of \name-BF}
\textbf{Notation:} Consider a standard partitioned Bloom filter with $m$ range, $\eta$ number of independent hashes. Let \name hash function be denoted by $\psi$ which, under the general construction in theorem \ref{thm:genconstruction}, is composed of LSH function $\phi$, and two RH functions $\rho_1, \rho_2$, also, the probability of collision between two tokens under $\phi$ hash function be denoted by $\zeta(x,y)$. Consider a sequence of tokens $\{x_1, x_2, ... x_n\}$ inserted into the \name-BF using hash function $\psi$ (in the proof $\psi = h$, $\mathcal{I}=\mathcal{H}$). 

\subsection{\name-BF without any assumptions}
The false positive rate $\epsilon$ of a query token $q$ can be written as follows where $p_q$ is false positive rate of one of the independent hashes.
\begin{equation}
    \epsilon = p_q^\eta
\end{equation}
We can write $p_q$ as
\begin{equation}
 p_q  = \mathbf{Pr}_{\h \leftarrow \mathcal{H}}(\bigvee_{i=1}^n \mathbf{1}(h(q) = h(x_i))
\end{equation}
 Using union bound on the probabilities of collision,

\begin{align*}
 p_q  \leq \sum_{i=1}^n \mathbf{Pr}_{h \leftarrow \mathcal{H}}(\mathbf{1}(h(q) = h(x_i)))\\
 = \sum_{i=1}^n \left( \frac{1}{L} \zeta(q, x_i) + (1 - \zeta(q, x_i)) \frac{\eta}{m} \right)
\end{align*}
$m'$ is the actual range where $m' = m/\eta$ in standard partition. Let $s$ be the average probability of collision of $\zeta(q, x_i)$ over all tokens 

\begin{align*}
 \epsilon = p_q^\eta  \leq \left( \frac{ns}{L} + (1 - s) \frac{n\eta}{m} \right)
\end{align*}

The above equation tells us that the false positive rate $\epsilon$ will depend on the similarity of the $q$ with the inserted tokens $\{x_i\}$. However, it is not very useful. The reason is , in the best possible scenario when $\zeta(q,x_i)=0$ for all $i$, i.e. $s=0$, the false positive rate we get is 
\begin{equation}
    \epsilon \leq \left( \frac{\eta n}{m} \right)^\eta
\end{equation}
If we compare this equation with false positive rate from the Bloom filter would be 
\begin{equation}
    \epsilon(\textrm{standard partitioned Bloom-filter}) = \left( 1 - \left( 1 - \frac{\eta}{m} \right)^n \right)^\eta \approx_{\textrm{first-order}} \left(\frac{\eta n}{m}\right)^\eta
\end{equation}

Thus the analysis we get without any assumptions is equivalent to the first order analysis of Bloom-filters which is far from the actual false positive rate of Bloom-filter.

\subsection{Realistic assumptions motivated from gene-search}
We make the following assumptions about the setup,
\begin{itemize}
    \item \textbf{A1:} $\zeta(x_i, x_j) = 0 \textrm{ if } |i - j| >= w_1$
    \item \textbf{A2:}$| \{x_i \; | \;  \zeta(q, x_i) > 0\}| \leq w_2$
\end{itemize}

\begin{lemma}
In gene-search, while using BF with k-mer size $k$ and sub-kmer size $t$, given assumption $A_1$ with $w_1=k$. the assumptions A2 is true with $w_2 = (k-t+1)^2$
\end{lemma}

Let us now compute false positive rate for one independent repetition.
\begin{align*}
 p_q  = \mathbf{Pr}_{h \leftarrow \mathcal{H}}\left(\bigvee_{i=1}^n \mathbf{1}(h(q) = h(x_i) \right) 
\end{align*}
Let $C = \{x_{i_j}\}_{j=1}^{w_2}$ be the tokens in the sequence which has non-zero collision probability with $q$
Also let us divide the tokens into sets of size $w_1$ ,
\begin{equation}
    X_i = \{x_{iw_i}, ... x_{(i+1)w_i}\}
\end{equation}
Let $\bar{X}_i$ be defined as 
\begin{equation}
    \bar{X}_i = \{x | x \in X_i \wedge x \notin C \}
\end{equation}

Then we can write,
\begin{align*}
 p_q  = \mathbf{Pr}_{h \leftarrow \mathcal{H}} \left( \left(\bigvee_{x \in C} \mathbf{1}(h(q) = h(x) \right)  \vee \left(\bigvee_{x \in \cup \bar{X}_{2i}} \mathbf{1}(h(q) = h(x) \right) \vee \left(\bigvee_{x \in \cup \Bar{X}_{2i+1}} \mathbf{1}(h(q) = h(x) \right)\right)
\end{align*}

Using union bound, we have 

\begin{align*}
 p_q  \leq \left( \left( \sum_{x \in C} \left(\frac{\zeta(x, q)}{L} + \frac{\eta}{m}\right) \right)  + \mathbf{Pr}_{h \leftarrow \mathcal{H}} \left(\bigvee_{x \in \cup \bar{X}_{2i}} \mathbf{1}(h(q) = h(x) \right) + \mathbf{Pr}_{h \leftarrow \mathcal{H}}  \left(\bigvee_{x \in \cup \Bar{X}_{2i+1}} \mathbf{1}(h(q) = h(x) \right)\right)
\end{align*}

Let $\{ h(X) = h(x) | x \in X \}$ We can write 

\begin{align*}
 p_q  \leq \left( \left( \sum_{x \in C} \left(\frac{\zeta(x, q)}{L} + \frac{\eta}{m}\right) \right)  + \mathbf{Pr}_{h \leftarrow \mathcal{H}} \left(\bigvee_{X=\bar{X}_{2i}} \mathbf{1}(h(q) \in h(X) \right) + \mathbf{Pr}_{h \leftarrow \mathcal{H}}  \left(\bigvee_{X=\bar{X}_{2i+1}} \mathbf{1}(h(q) \in h(X) \right)\right)
\end{align*}

\begin{lemma}
For distinct $i$ and $j$, the events of the type $\mathbf{1}(h(q) \in X_{2i})$ and  $\mathbf{1}(h(q) \in X_{2j})$ are independent. The events of the type $\mathbf{1}(h(q) \in X_{2i+1})$ and  $\mathbf{1}(h(q) \in X_{2j+1})$ are independent. 
\end{lemma}
Thus, we can write

\begin{align*}
 p_q  \leq  \sum_{x \in C} \left(\frac{\zeta(x, q)}{L} + \frac{\eta}{m} \right)   + \left( 1 -  \mathbf{Pr}_{h \leftarrow \mathcal{H}} \left( \bigwedge_{X=\bar{X}_{2i}} \mathbf{1}(h(q) \notin h(X) \right) \right)+ \left( 1 - \mathbf{Pr}_{h \leftarrow \mathcal{H}}  \left(\bigwedge_{X=\bar{X}_{2i+1}} \mathbf{1}(h(q) \notin h(X) \right)\right)
\end{align*}

\begin{align*}
 p_q  \leq  \sum_{x \in C} \left(\frac{\zeta(x, q)}{L} + \frac{\eta}{m} \right)   + \left( 1 -  \prod_{X=\bar{X}_{2i}} \mathbf{Pr}_{h \leftarrow \mathcal{H}} \left( \mathbf{1}(h(q) \notin h(X) \right) \right)  + \left( 1 -  \prod_{X=\bar{X}_{2i+1}} \mathbf{Pr}_{h \leftarrow \mathcal{H}} \left( \mathbf{1}(h(q) \notin h(X) \right) \right)
\end{align*}

\begin{align*}
 p_q  \leq  \sum_{x \in C} \left(\frac{\zeta(x, q)}{L} + \frac{\eta}{m} \right)   + \left( 1 -  \prod_{X=\bar{X}_{2i}} \left( 1 - \mathbf{Pr}_{h \leftarrow \mathcal{H}} \left( \mathbf{1}(h(q) \in h(X) \right) \right) \right)   + \left( 1 -  \prod_{X=\bar{X}_{2i+1}} \left( 1 - \mathbf{Pr}_{h \leftarrow \mathcal{H}} \left( \mathbf{1}(h(q) \in h(X) \right) \right) \right)
\end{align*}
Applying union bound within sets,

\begin{align*}
 p_q  \leq  \sum_{x \in C} \left(\frac{\zeta(x, q)}{L} + \frac{\eta}{m} \right)   + \left( 1 -  \prod_{X=\bar{X}_{2i}} \left( 1 - \sum_{x \in X} \mathbf{Pr}_{h \leftarrow \mathcal{H}} \left( \mathbf{1}(h(q) = h(x) \right) \right) \right)   + \left( 1 -  \prod_{X=\bar{X}_{2i+1}} \left( 1 - \sum_{x \in X} \mathbf{Pr}_{h \leftarrow \mathcal{H}} \left( \mathbf{1}(h(q) = h(x) \right) \right) \right) 
\end{align*}

By replacing $\bar{X}_i$ with $X$, we only increase the RHS. Hence,

\begin{align*}
 p_q  \leq  \sum_{x \in C} \left(\frac{\zeta(x, q)}{L} + \frac{\eta}{m} \right)   + \left( 1 -  \prod_{X=X_{2i}} \left( 1 - \sum_{x \in X} \mathbf{Pr}_{h \leftarrow \mathcal{H}} \left( \mathbf{1}(h(q) = h(x) \right) \right) \right)   + \left( 1 -  \prod_{X=X_{2i+1}} \left( 1 - \sum_{x \in X} \mathbf{Pr}_{h \leftarrow \mathcal{H}} \left( \mathbf{1}(h(q) = h(x) \right) \right) \right) 
\end{align*}

\begin{align*}
 p_q  \leq  \sum_{x \in C} \left(\frac{\zeta(x, q)}{L} + \frac{\eta}{m} \right)   + \left( 1 -  \prod_{X=X_{2i}} \left( 1 - \sum_{x \in X} \left( \frac{\eta}{m} \right) \right) \right)   + \left( 1 -  \prod_{X=X_{2i+1}} \left( 1 - \sum_{x \in X} \left( \frac{\eta}{m} \right) \right) \right) 
\end{align*}
It follows,

\begin{align*}
 p_q  \leq  \sum_{x \in C} \left(\frac{\zeta(x, q)}{L} + \frac{\eta}{m} \right)   + 2 \left( 1 -  \left( 1 - \left( \frac{w_1\eta}{m} \right) \right)^{\frac{n}{2w_1}} \right) 
\end{align*}

$\zeta(x,q) \leq 1$

\begin{align*}
 p_q  \leq  w_2\left(\frac{1}{L} + \frac{\eta}{m} \right)   + 2 \left( 1 -  \left( 1 - \left( \frac{w_1\eta}{m} \right) \right)^{\frac{n}{2w_1}} \right) 
\end{align*}

Thus the false positive rates are bounded by

\begin{align*}
\epsilon  \leq \left( w_2\left(\frac{1}{L} + \frac{\eta}{m} \right)   + 2 \left( 1 -  \left( 1 - \left( \frac{w_1\eta}{m} \right) \right)^{\frac{n}{2w_1}} \right) \right)^\eta
\end{align*}
\begin{align*}
\epsilon  \leq \left( w_2\left(\frac{1}{L} + \frac{\eta}{m} \right)   + 2 \left( 1 -  \left( 1 - \left( \frac{w_1\eta}{m} \right) \right)^{\frac{n}{2w_1}} \right) \right)^\eta
\approx \left( w_2\left(\frac{1}{L} + \frac{\eta}{m} \right)   + 2 \left( 1 -  e^{-\frac{\eta n}{2m}}  \right) \right)^\eta
\end{align*}

Note for a given $\eta$, the if $m\rightarrow \infty$, the $\epsilon$ is upper bounded by $(\frac{w_2}{L})^\eta$.  For large enough $L$ and a reasonable value of $\eta$, this bound is also very small.

\section{Proof of lemma 1}
\begin{proof} 
Any query k-mer can have at most $(k-t+1)$ sub-k-mers and each of these sub-kmers can be part of at most $(k-t+1)$ k-mers in the data. Hence, there can be atmost $(k-t+1)^2$ k-mers that have non-zero Jaccard similarity and hence the probability of collision with query k-mer
\end{proof}

\section{\name hash code}
Get the murmur hash code from \cite{murmur}.

\begin{verbatim}
#ifndef _HASHER_H_
#define _HASHER_H_

#include <iostream>
#include <string>
#include "MurmurHash3.h"
#include <assert.h>
#include <cmath>
using namespace std;

class Hasher {
protected:
    const char *sequence;
    size_t sequence_len;
    const uint64_t range;
    const uint32_t num_hashes;
    const uint32_t seed;
    uint32_t pos;
    uint64_t RANGEMASK;
public:
    Hasher(uint64_t range, uint32_t num_hashes, uint32_t seed=0)
        : range(range), num_hashes(num_hashes), seed(seed), pos(0) {

        uint64_t Rbits = (int)std::log2((float) range);
        RANGEMASK = (1LL<<Rbits) -1;
    }

    inline bool hasNext() {
        return pos <= sequence_len - 31;
    }

    uint32_t nHashesInSequence() {
        return sequence_len - 30;
    }

    virtual void hash(uint64_t * out) = 0;

    void setSequence(const string & _sequence) {
        sequence = _sequence.data();
        sequence_len = _sequence.size();
        pos = 0;
    }
};

class MurmurHasher : public Hasher {
public:
    MurmurHasher(uint64_t range, uint32_t num_hashes, uint32_t seed=0)
        : Hasher(range, num_hashes, seed) {}

    void hash(uint64_t * out) override {
        for (uint32_t j = 0; j < num_hashes; ++j) {
            MurmurHash3_x64_64(sequence + pos, 31, seed + j, out + j);
            out[j] = out[j]  & RANGEMASK;
        }
        pos += 1;
    }
};

static uint32_t next_pow_of_2(uint32_t x) {
    uint32_t power = 1;
    while (power < x) {
        power *= 2;
    }
    return power;
}

class EfficientIDLHasher : public Hasher {
protected:
    const uint32_t kMer;
    const uint32_t universalHashRange;
    uint32_t tree_length;
    uint64_t *trees;
    uint32_t index_to_pop;
    uint64_t* oneperm_hash_helper_arr = new uint64_t [33];
    int32_t Lbits;
    uint64_t URANGEMASK;
public:
    EfficientIDLHasher(uint64_t range, uint32_t num_hashes, uint32_t kMer, uint32_t universalHashRange, uint32_t seed=0)
        : Hasher(range, num_hashes, seed), kMer(kMer), universalHashRange(universalHashRange),
          tree_length(next_pow_of_2(32 - kMer) * 2 - 1), trees(new uint64_t[tree_length * num_hashes]), index_to_pop(0) {
        fill(trees, trees + tree_length * num_hashes, UINT64_MAX);
        Lbits = (int)std::log2((float) universalHashRange);
        URANGEMASK = (1LL<<Lbits) -1;
        std::cout << "Lbits: " << Lbits << "urange: " << universalHashRange << std::flush << std::endl;
        assert(num_hashes*Lbits <= 64);  // can be increased if required
    }

    void buildTrees() {
        uint32_t idx1;
        for (uint32_t i = 0; i < num_hashes; ++i) {
            idx1 = tree_length * i;
            for (int32_t j = tree_length / 2 - 1; j >= 0; --j) {
                trees[idx1 + j] = min(
                    trees[idx1 + j * 2 + 1],
                    trees[idx1 + j * 2 + 2]
                );
            }
        }
    }

    void hash(uint64_t * out) override {
        uint64_t hashValue, minValue, uhashvalue;
        uint32_t i, j, new_index;
        uint32_t idx1;
        //uint32_t seed1;
        uint64_t one_perm_shift = UINT64_MAX / num_hashes;
        MurmurHash3_x64_64(sequence + pos, 31, seed, &uhashvalue);
        if (pos == 0) {
            // initial tree construction
            for (j=0; j<=32 - kMer; ++j) {
                MurmurHash3_x64_64(sequence + pos + j, kMer, seed, &oneperm_hash_helper_arr[j]);
            }

            for (i = 0; i < num_hashes; ++i) {
                minValue = UINT64_MAX;
                idx1 = tree_length * i + tree_length / 2;
                //seed1 = seed + i;
                for (j = 0; j <= 31 - kMer; ++j) {
                    hashValue = oneperm_hash_helper_arr[j] - i*one_perm_shift;
                    minValue = min(hashValue, minValue);
                    trees[idx1 + j] = hashValue;
                }
                //MurmurHash3_x64_64(sequence + pos, 31, seed1, out + i, universalHashRange);
                out[i] = (uhashvalue >> (i*Lbits)) & URANGEMASK;
                out[i] += minValue & RANGEMASK;
            }
            buildTrees();
            index_to_pop = 0;
        } else {
            MurmurHash3_x64_64(sequence + pos + 31 - kMer, kMer, seed, &oneperm_hash_helper_arr[0]);
            for (i = 0; i < num_hashes; ++i) {
                hashValue = (oneperm_hash_helper_arr[0] -i*one_perm_shift);
                new_index = tree_length / 2 + index_to_pop;
                //seed1 = seed + i;
                idx1 = tree_length * i;
                trees[idx1 + new_index] = hashValue;
                while (new_index > 0) {
                    new_index = (new_index - 1) / 2;
                    trees[idx1 + new_index] = min(
                        trees[idx1 + new_index * 2 + 1],
                        trees[idx1 + new_index * 2 + 2]
                    );
                }
                //MurmurHash3_x64_64(sequence + pos, 31, seed1, out + i, universalHashRange);
                out[i] = (uhashvalue >> (i*Lbits)) & URANGEMASK;
                out[i] += trees[idx1] & RANGEMASK;
            }
            index_to_pop = (index_to_pop + 1) % (32 - kMer);
        }
        pos += 1;
    }
};

#endif


\end{verbatim}
